# Supplementary material for: On the inclusion of non-concurrent controls in platform trials with an interim analysis
Source: arXiv:2509.08795 source file (2026-03-24)
Supplement: Supplementary file 1 [file Suppmaterial.pdf]

# Supplementary material for “On the inclusion of non-concurrent controls in platform trials with a futility interim analysis”

Pavla Krotka<sup>1</sup>, Martin Posch<sup>2</sup>, and Marta Bofill Roig<sup>\*1</sup>

<sup>1</sup>*Department of Statistics and Operations Research and Institute for Research and Innovation in Health (IRIS),  
Universitat Politècnica de Catalunya, Barcelona, Spain*

<sup>2</sup>*Center for Medical Data Science, Medical University of Vienna, Vienna, Austria*

## A Additional results from the simulation study

For all subfigures indicated by **A)-D)**, the following design parameters were varied in the simulation:

**A)** Varying futility bound ( $\alpha_1$ ). These figures correspond to a platform trial with sample sizes per arm and period set to 150.

**B)** Varying ratio between the sample sizes in period 1 and period 2 ( $r$ ), where the period 2 sample sizes per arm are fixed. Sample sizes per arm in period 1 are determined by the chosen ratio  $r$ , i.e., increase or decrease with respect to the period 2 sample sizes  $r$ -times. These figures correspond to a platform trial with sample sizes per arm in period 2 set to 150, using a futility bound  $\alpha_1 = 0.5$ .

**C)** Varying ratio between the sample sizes in Arm 1 and control ( $a$ ), where the control arm sample sizes per period are fixed. Sample sizes in Arm 1 per period are determined by the chosen ratio  $a$ , i.e., increase or decrease with respect to the control arm sample sizes  $a$ -times. These figures correspond to a platform trial with sample sizes in the control arm per period set to 150, using a futility bound  $\alpha_1 = 0.5$ .

**D)** Varying strength of the time trend ( $\lambda$ ). These figures correspond to a platform trial with sample sizes per arm and period set to 150, using a futility bound  $\alpha_1 = 0.5$ .

---

\*marta.bofill.roig@upc.edu

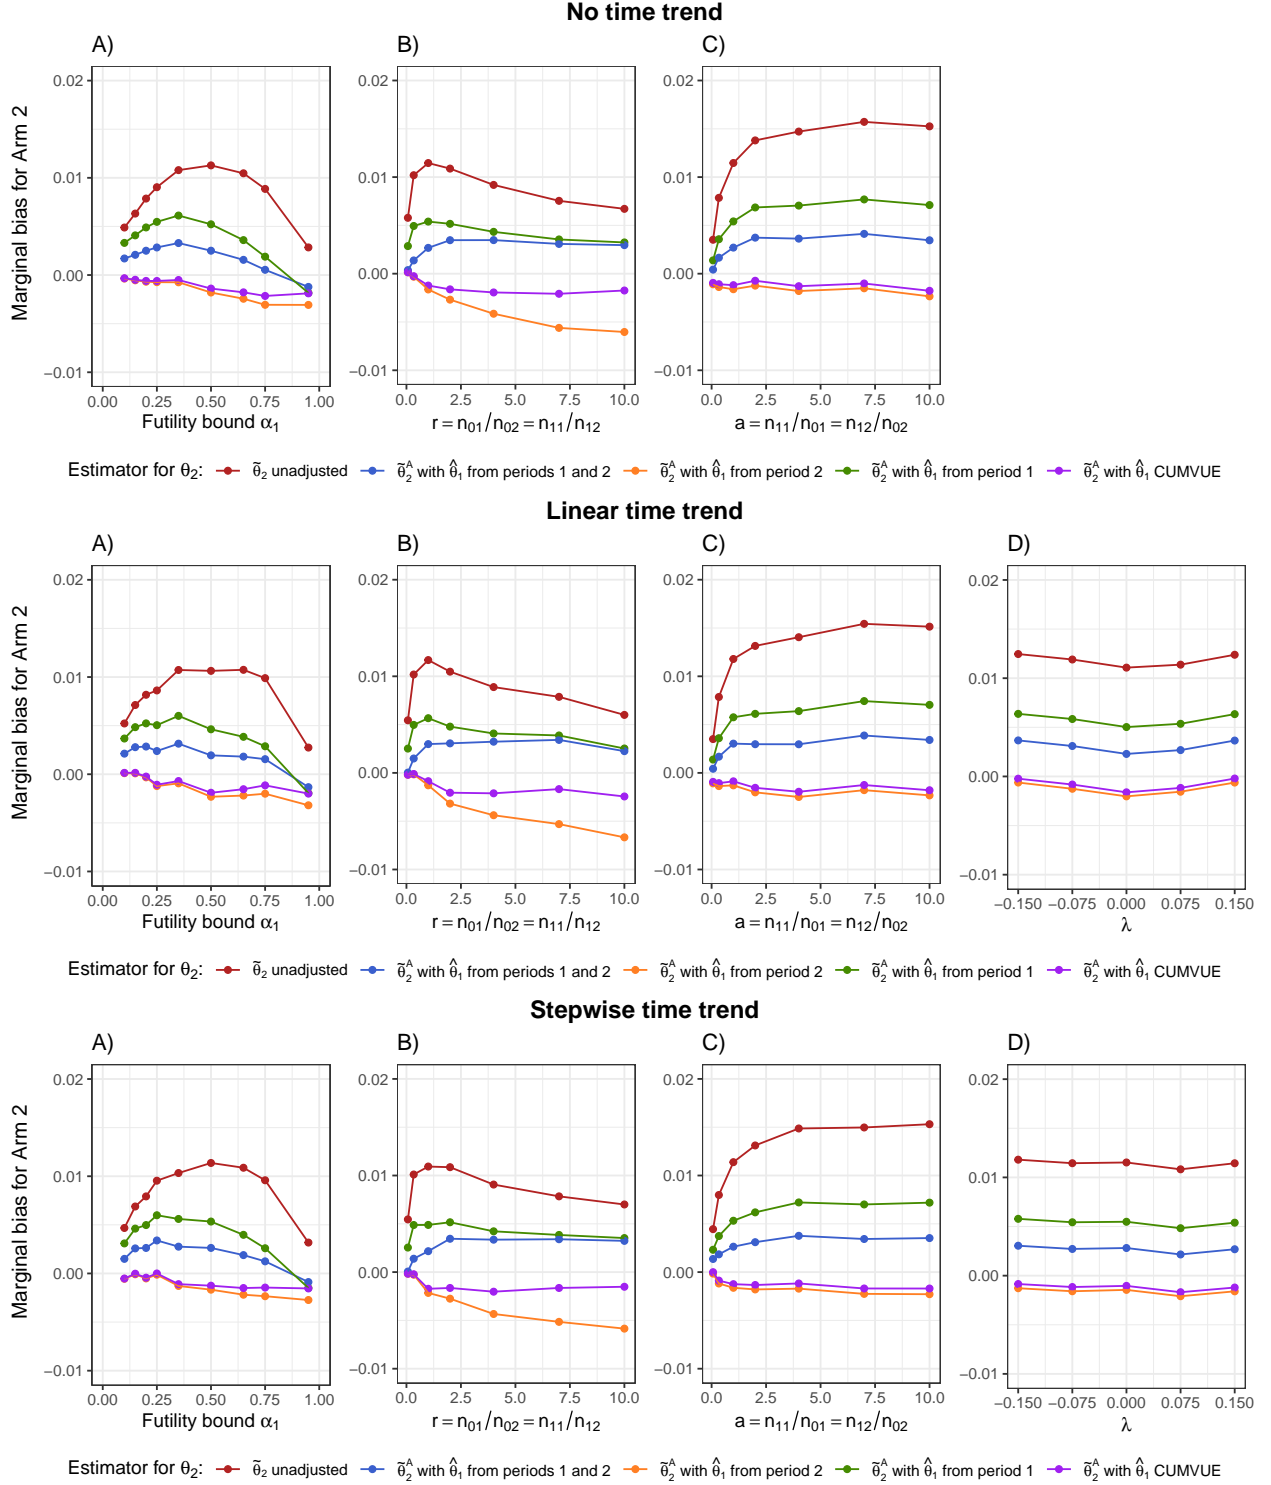

Figure S1: Marginal bias in the treatment effect estimator for Arm 2 using the unadjusted estimator  $\tilde{\theta}_2$  and the mean adjusted estimator  $\tilde{\theta}_2^A$  with  $\theta_1$  estimated from both periods, only period 1, only period 2, or using the CUMVUE. Results for scenarios under no time trend (first row), as well as linear (second row) and stepwise (third row) time trends are presented. In scenarios under time trends presented in figures A)-C), the time trend strength was set to  $\lambda = 0.15$ .

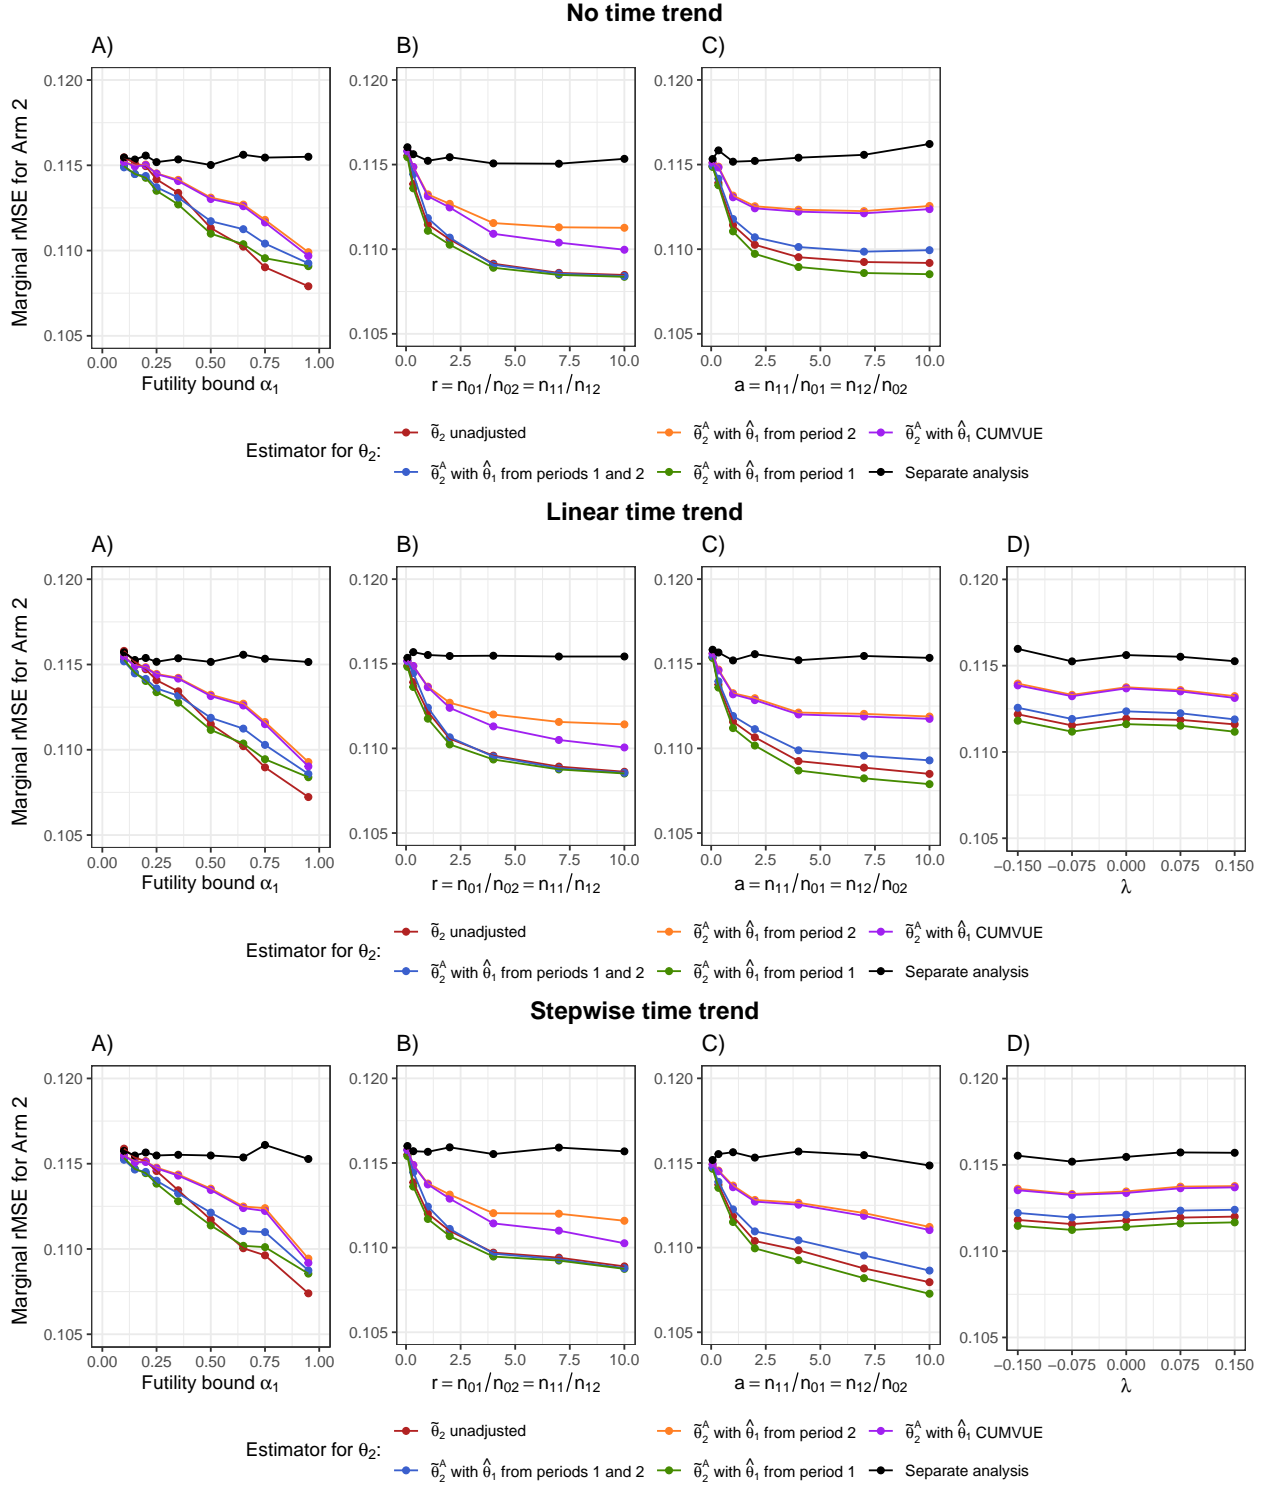

Figure S2: Marginal root mean squared error of the treatment effect estimator for Arm 2 using the unadjusted estimator  $\tilde{\theta}_2$  and the mean adjusted estimator  $\tilde{\theta}_2^A$  with  $\theta_1$  estimated from both periods, only period 1, only period 2, or using the CUMVUE. Results for scenarios under no time trend (first row), as well as linear (second row) and stepwise (third row) time trends are presented. In scenarios under time trends presented in figures A)-C), the time trend strength was set to  $\lambda = 0.15$ .

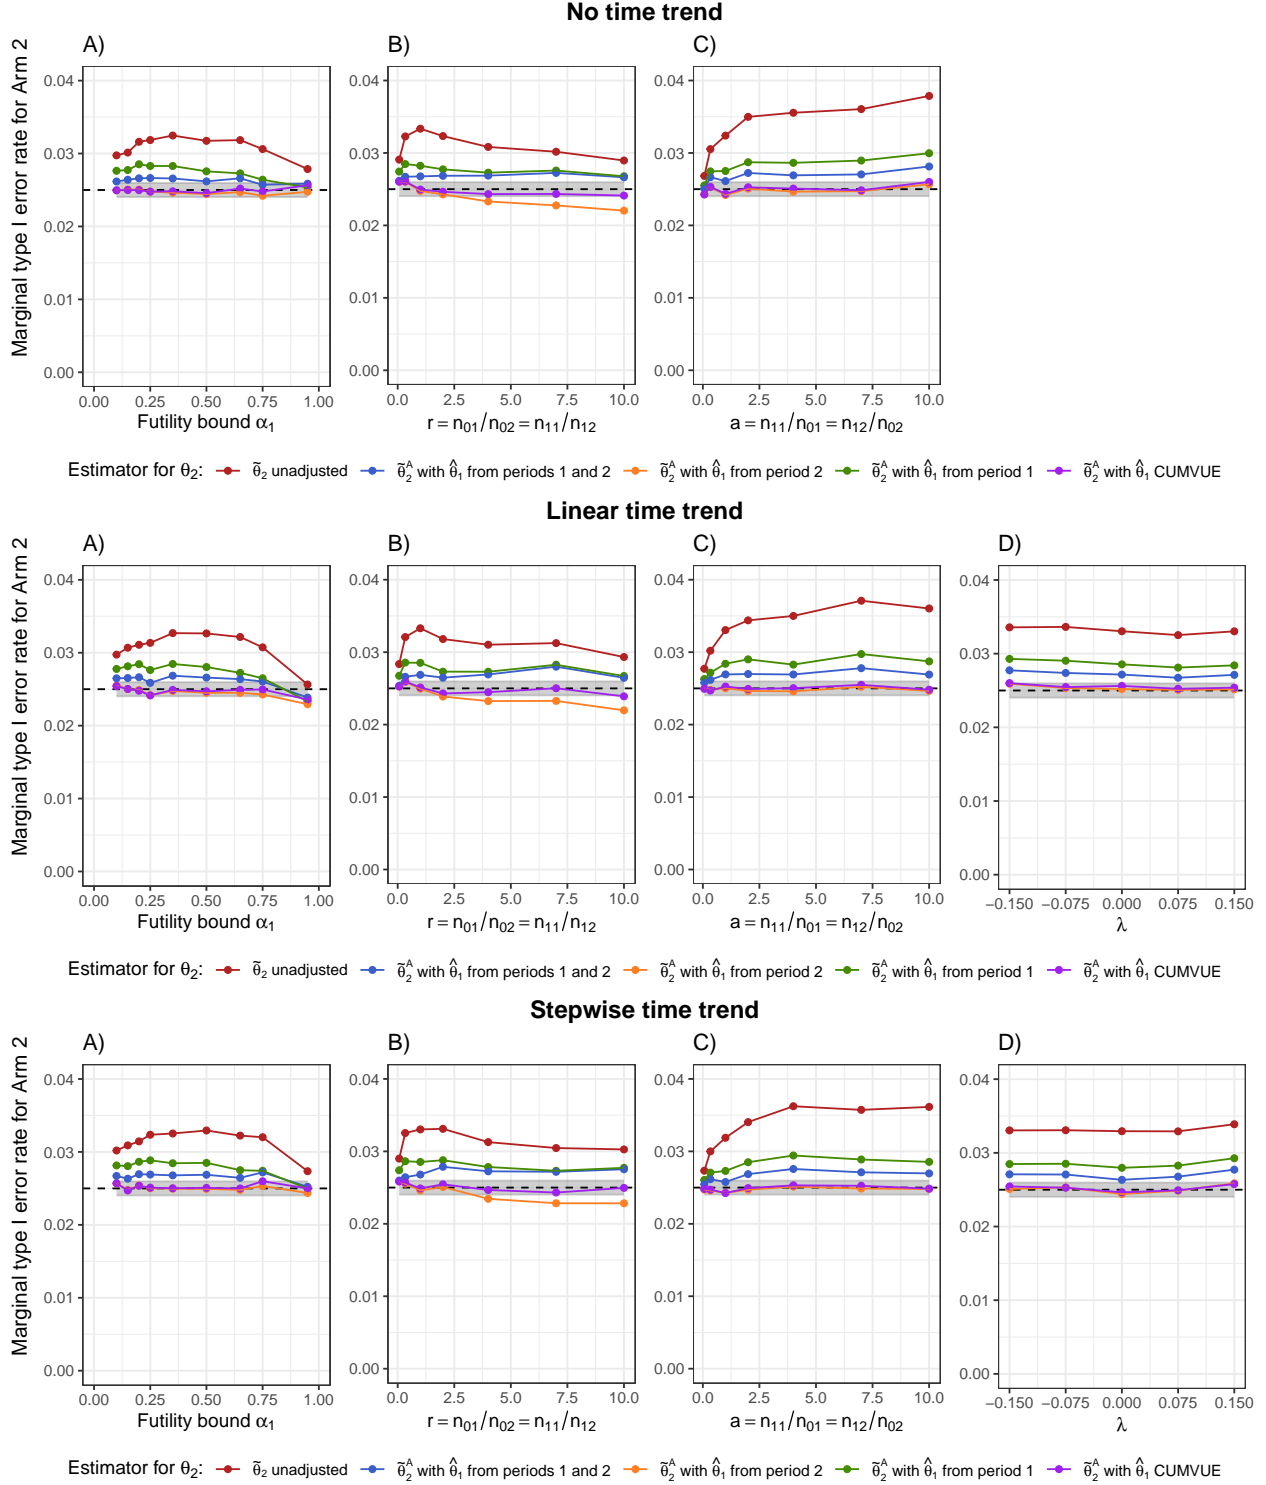

Figure S3: Marginal type I error rate for Arm 2 using the unadjusted estimator  $\tilde{\theta}_2$  and the mean adjusted estimator  $\tilde{\theta}_2^A$  with  $\theta_1$  estimated from both periods, only period 1, only period 2, or using the CUMVUE. Results for scenarios under no time trend (first row), as well as linear (second row) and stepwise (third row) time trends are presented. All figures include a dashed reference line for the nominal significance level of 0.025 and the simulation error is shown as a gray area representing the 95% confidence interval of the simulated type I error rate. In scenarios under time trends presented in figures A)-C), the time trend strength was set to  $\lambda = 0.15$ .

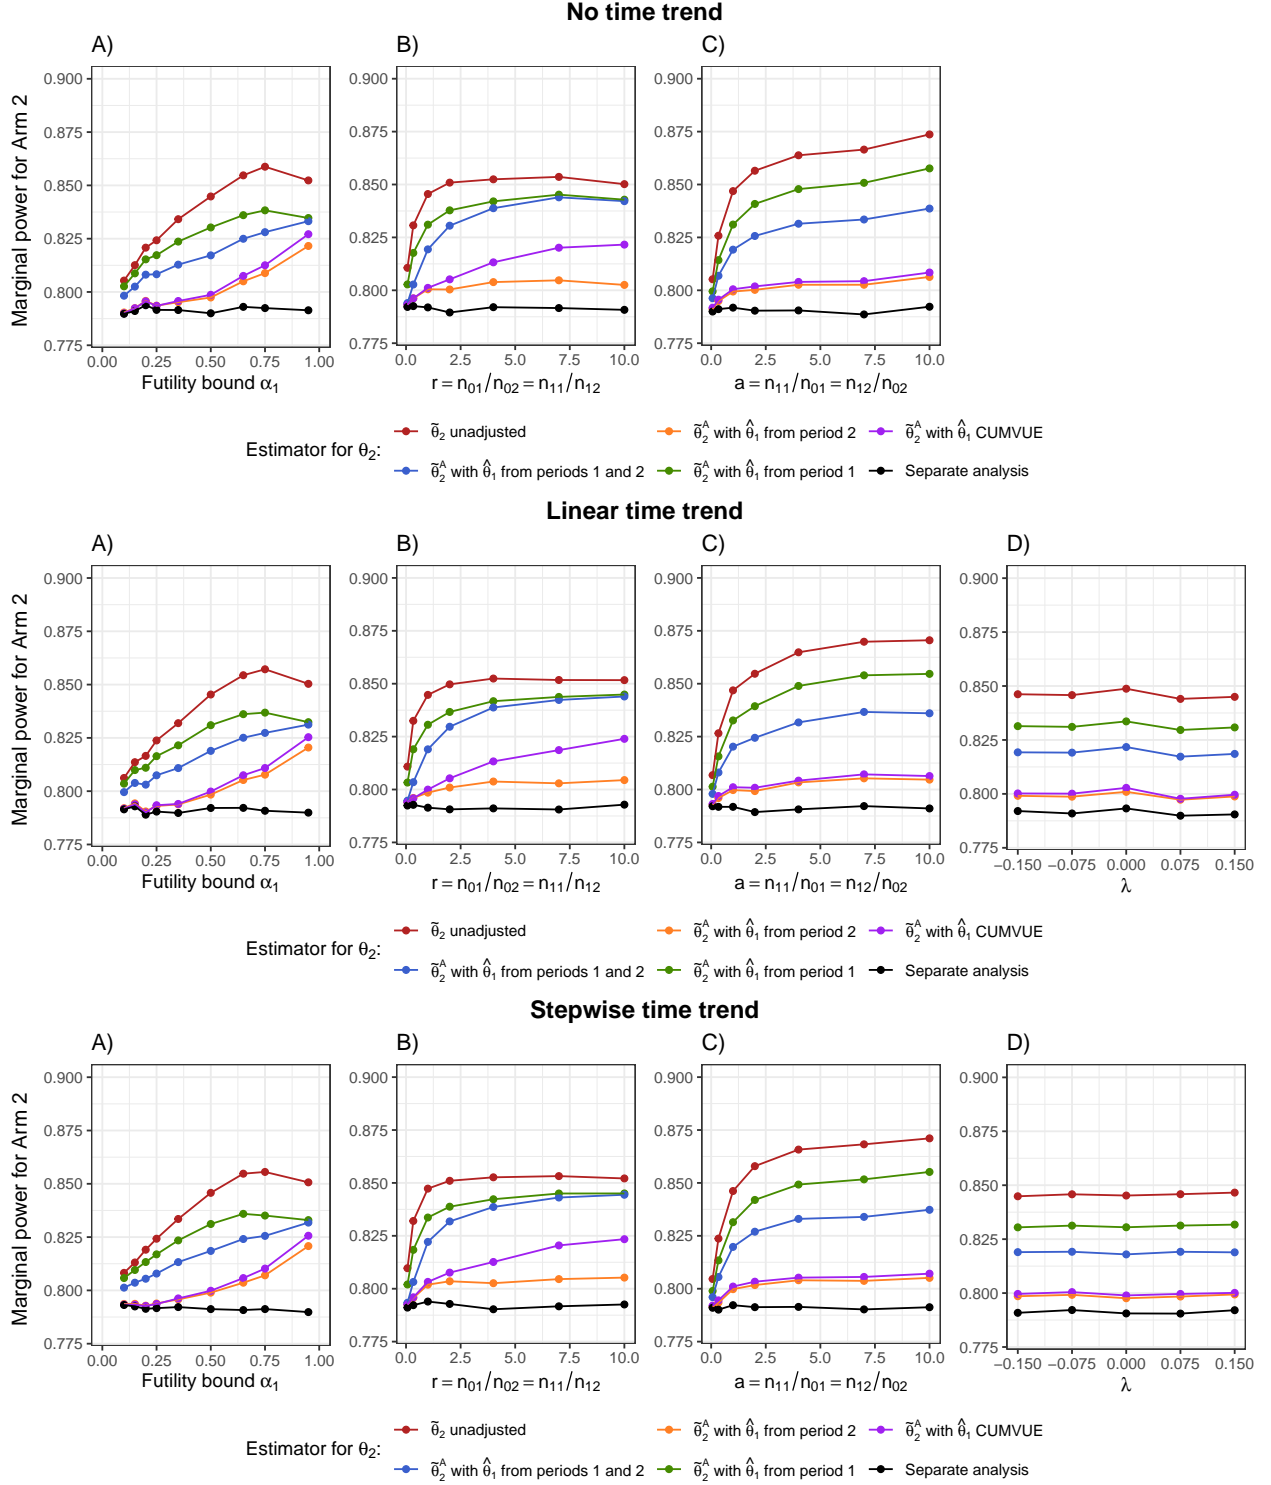

Figure S4: Marginal power for Arm 2 using the unadjusted estimator  $\tilde{\theta}_2$  and the mean adjusted estimator  $\tilde{\theta}_2^A$  with  $\theta_1$  estimated from both periods, only period 1, only period 2, or using the CUMVUE. Results for scenarios under no time trend (first row), as well as linear (second row) and stepwise (third row) time trends are presented. In scenarios under time trends presented in figures A)-C), the time trend strength was set to  $\lambda = 0.15$ .

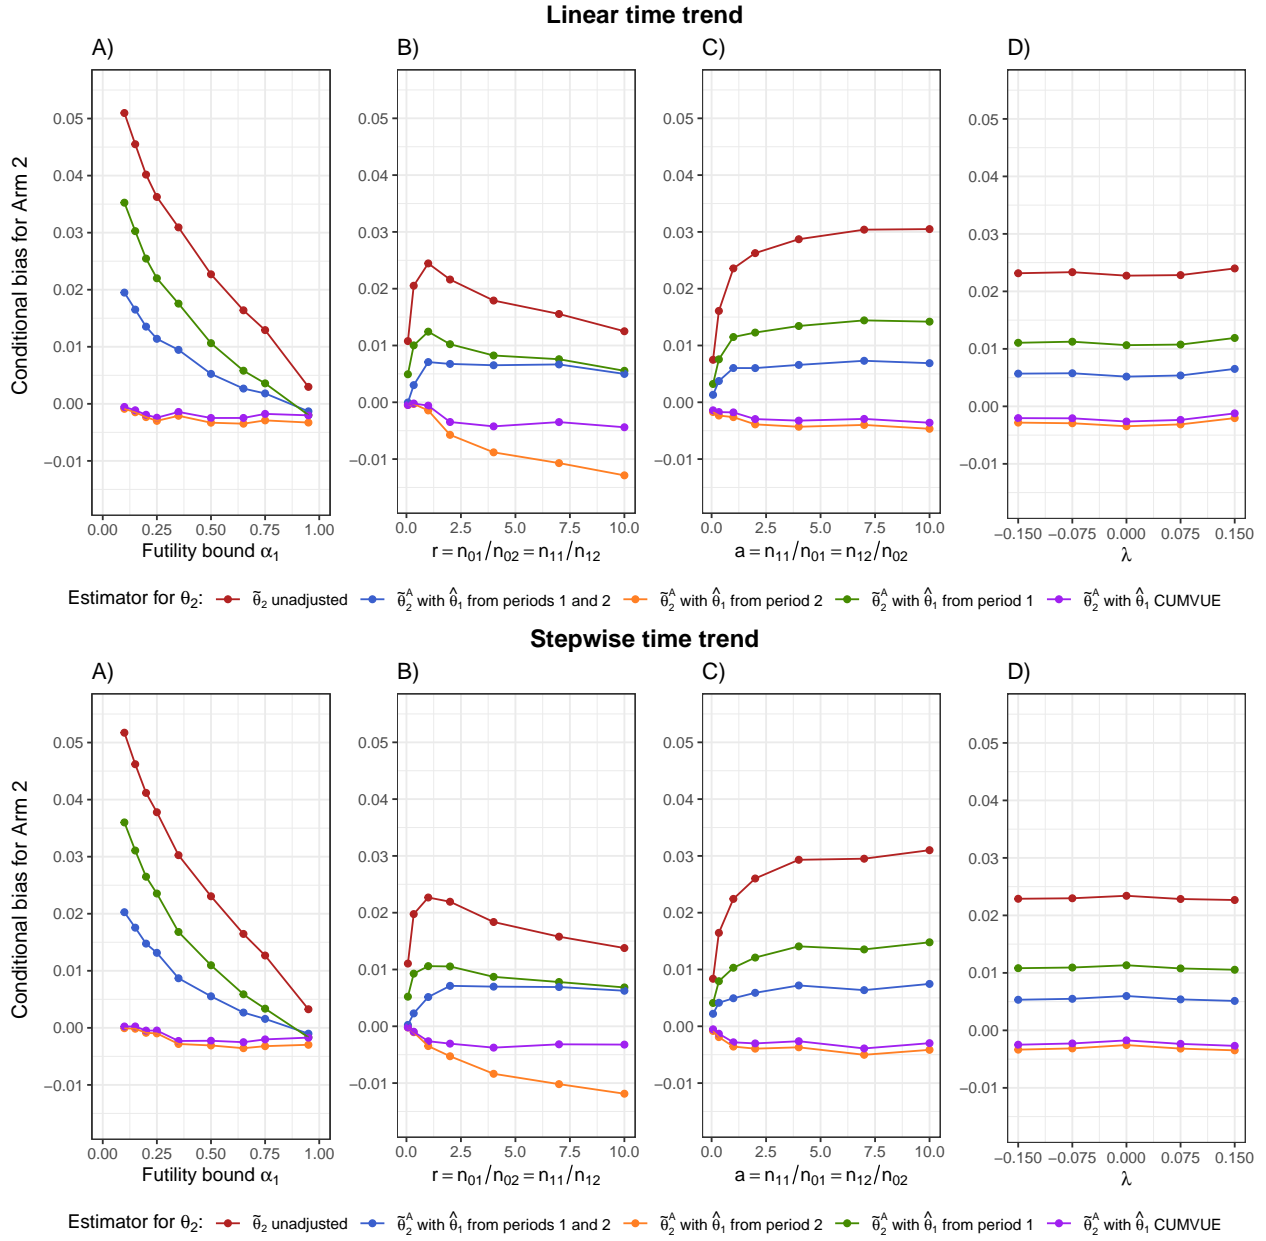

Figure S5: Conditional bias in the treatment effect estimator for Arm 2 using the unadjusted estimator  $\tilde{\theta}_2$  and the mean adjusted estimator  $\tilde{\theta}_2^A$  with  $\theta_1$  estimated from both periods, only period 1, only period 2, or using the CUMVUE. Results for scenarios under linear (first row) and stepwise (second row) time trends are presented. In scenarios presented in figures A)-C), the time trend strength was set to  $\lambda = 0.15$ .

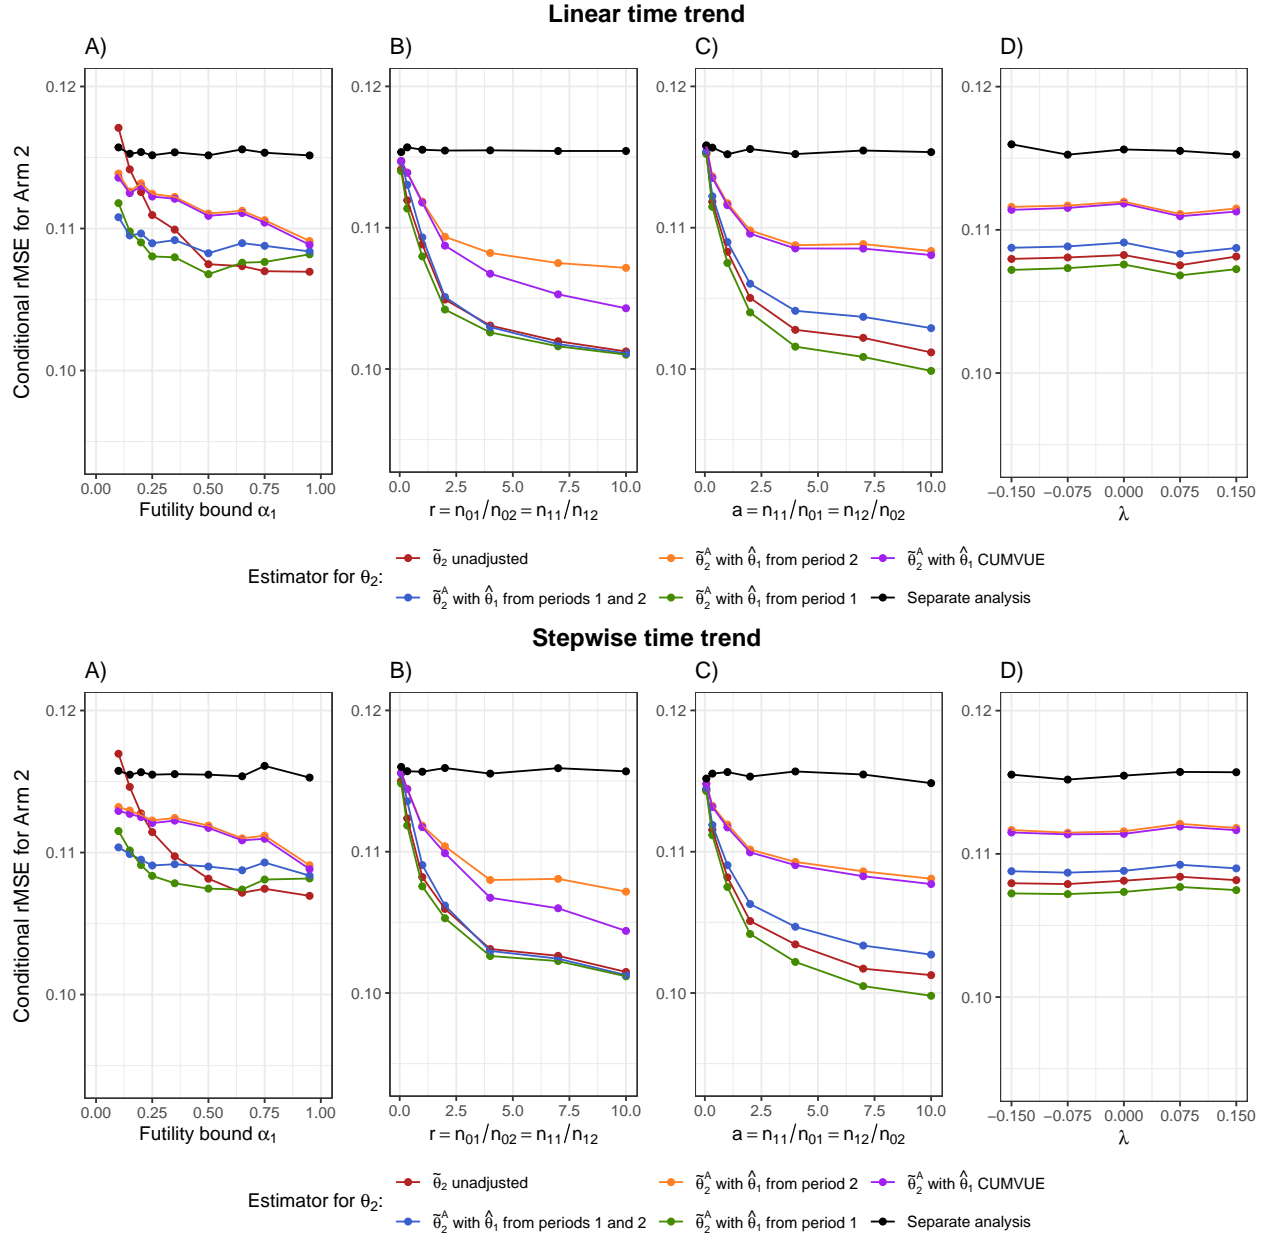

Figure S6: Conditional root mean squared error of the treatment effect estimator for Arm 2 using the unadjusted estimator  $\tilde{\theta}_2$  and the mean adjusted estimator  $\tilde{\theta}_2^A$  with  $\theta_1$  estimated from both periods, only period 1, only period 2, or using the CUMVUE. Results for scenarios under linear (first row) and stepwise (second row) time trends are presented. In scenarios presented in figures A)-C), the time trend strength was set to  $\lambda = 0.15$ .

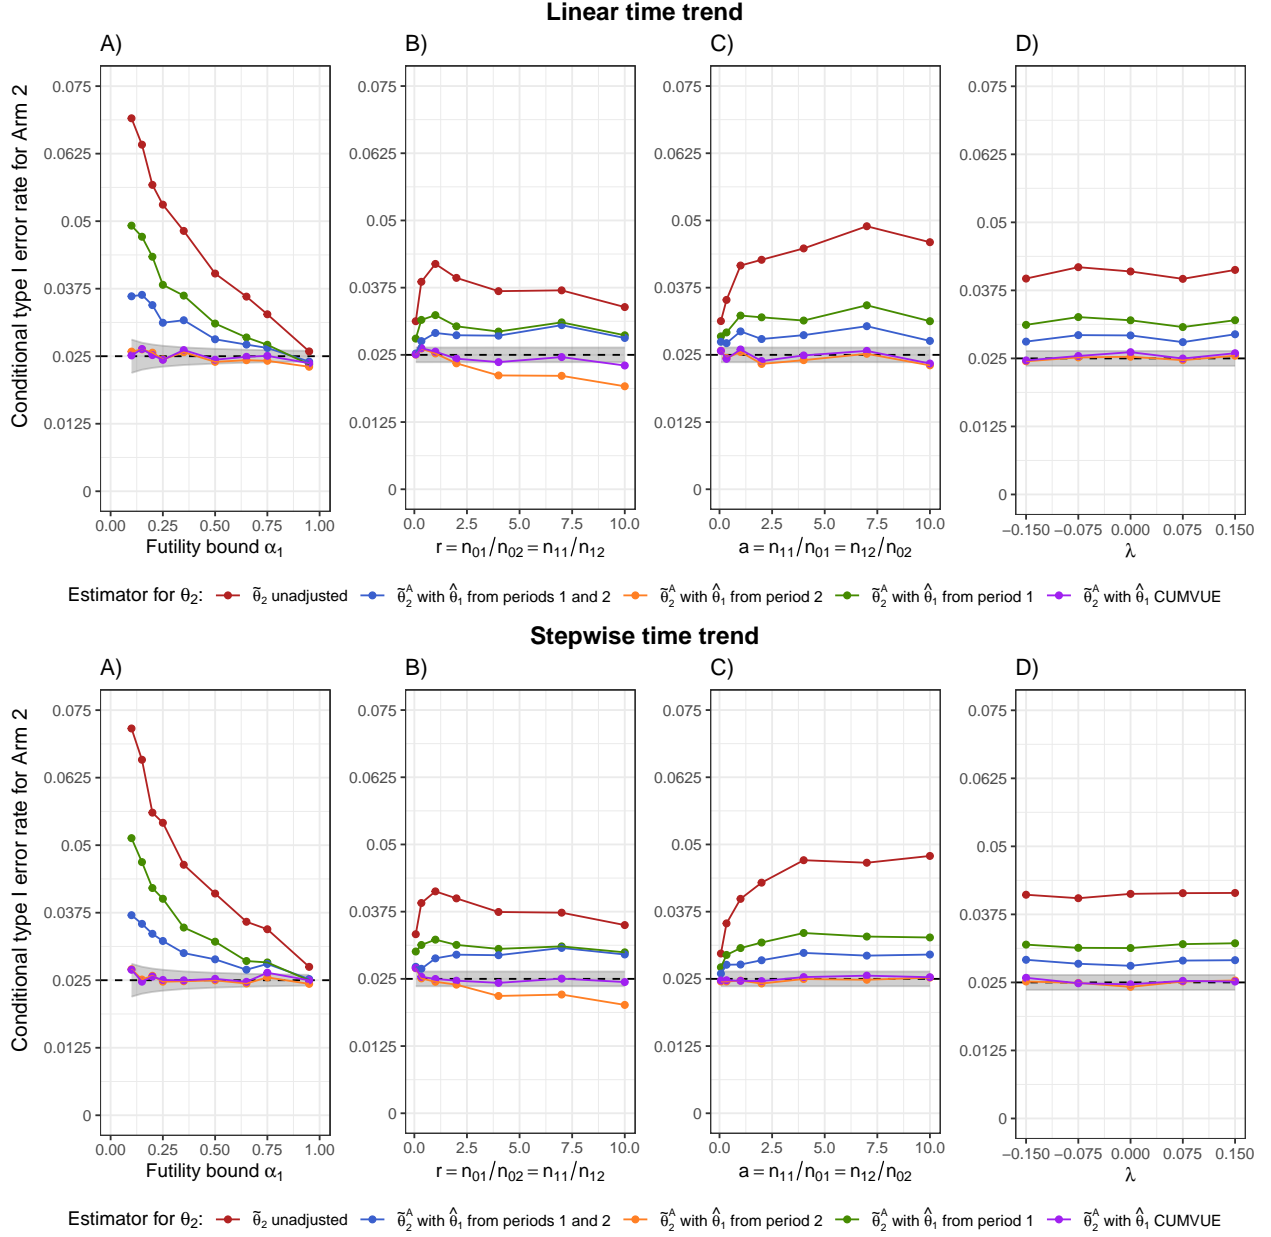

Figure S7: Conditional type I error rate for Arm 2 using the unadjusted estimator  $\tilde{\theta}_2$  and the mean adjusted estimator  $\hat{\theta}_2$  and the mean adjusted estimator  $\hat{\theta}_2^A$  with  $\theta_1$  estimated from both periods, only period 1, only period 2, or using the CUMVUE. Results for scenarios under linear (first row) and stepwise (second row) time trends are presented. All figures include a dashed reference line for the nominal significance level of 0.025 and the simulation error is shown as a gray area representing the 95% confidence interval of the simulated type I error rate. In scenarios presented in figures A)-C), the time trend strength was set to  $\lambda = 0.15$ .

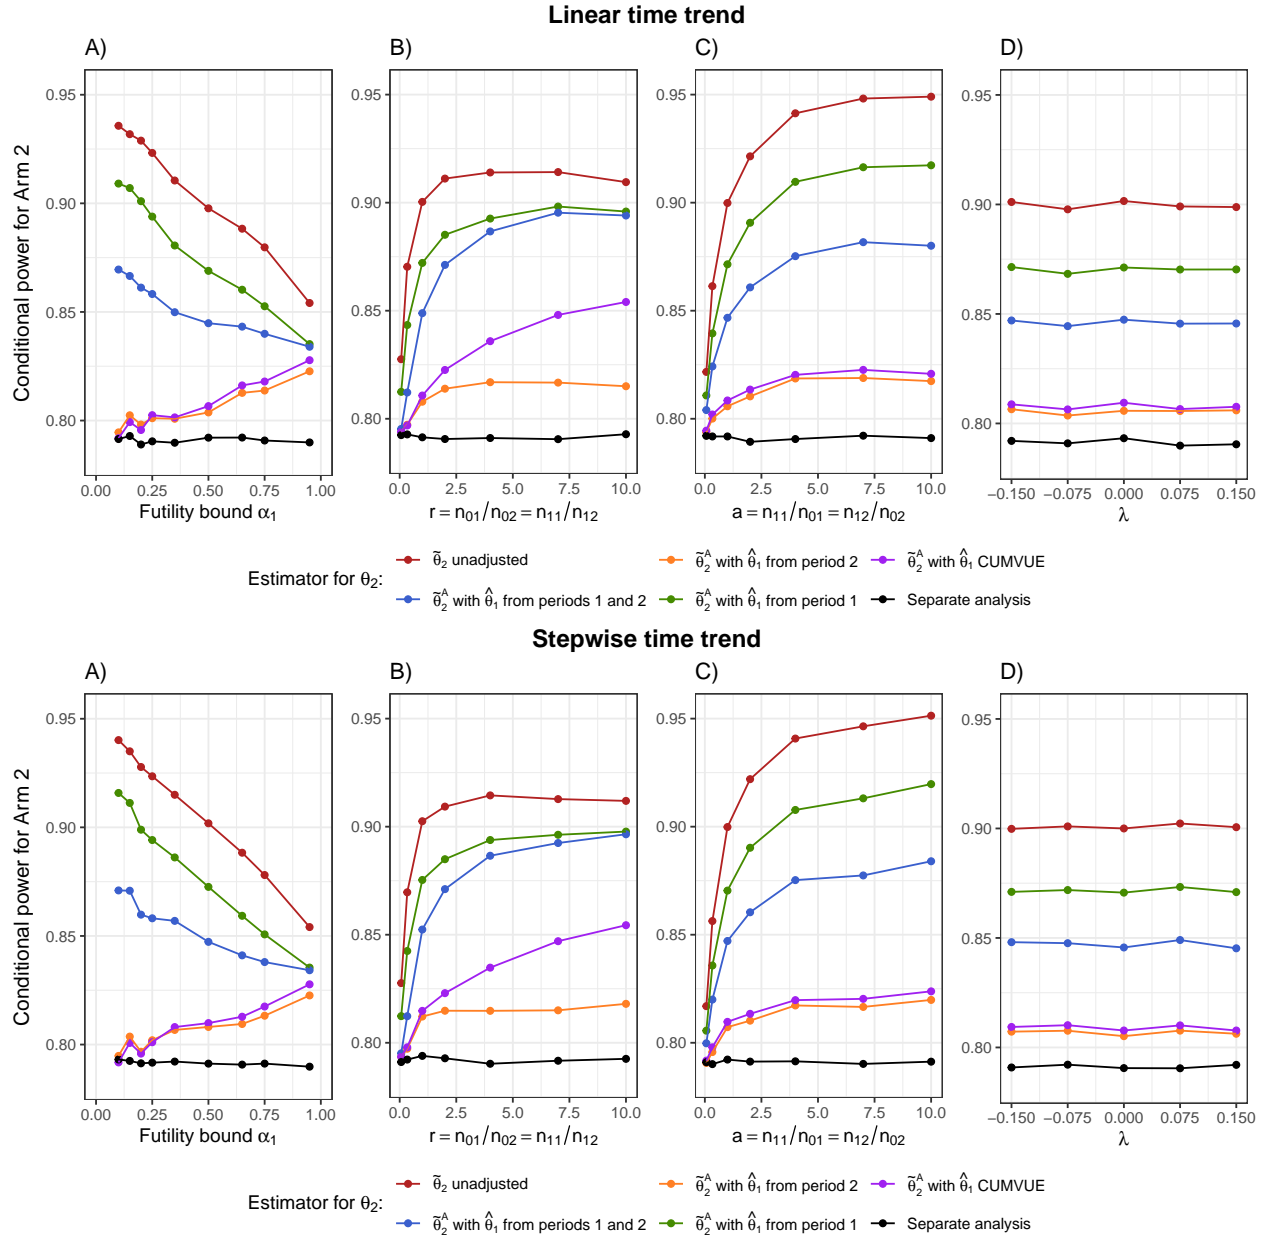

Figure S8: Conditional power for Arm 2 using the unadjusted estimator  $\tilde{\theta}_2$  and the mean adjusted estimator  $\tilde{\theta}_2^A$  with  $\theta_1$  estimated from both periods, only period 1, only period 2, or using the CUMVUE. Results for scenarios under linear (first row) and stepwise (second row) time trends are presented. In scenarios presented in figures A)-C), the time trend strength was set to  $\lambda = 0.15$ .
